# Supplementary material for: Trainable amorphous matter: tuning yielding by mechanical annealing
Source: arXiv:2512.01019 source file (2025-11-30)
Supplement: Supplementary file 1 [file SI.pdf]

# Supplementary Information for *Trainable amorphous matter*: tuning yielding by mechanical annealing

## S1 Method of identifying yield strain, shear modulus and the degree of brittleness ( $\gamma_Y$ , $\tilde{G}$ , $\tilde{m}$ ):

We have used the normalized differential modulus  $G/G_0$ , where  $G = d\sigma/d\gamma$  and  $G_0 = G(t=0)$ , to identify the yield strain. The  $G/G_0$  vs.  $\gamma$  curves exhibit a sharp change in slope at yielding. To determine the value of the yield strain quantitatively, two small regions—one before the drop and one just beyond it, were fitted linearly, and the intersection of the two fits is taken as the yield strain. Fig. S1(a)–(d) shows this procedure for  $\gamma_T = 0.04, 0.10, 0.18$ , and  $0.30$ , respectively, in experiments. Similar algorithms have been used in the case of simulations as well.

To calculate the linear modulus, we determined the slope of the stress–strain curve ( $\sigma$  vs.  $\gamma$ ) up to  $\gamma = \gamma_Y/2$ , as shown in Fig. S1(e–h) for the experiments. The same procedure was applied to the simulation data. For comparison across all cases, the linear modulus  $G_{\text{linear}}$  was normalized by the corresponding value obtained for the poorly annealed system ( $G_{\text{ref}}$ ), defining the normalized linear modulus as  $\tilde{G} = G_{\text{linear}}/G_{\text{ref}}$ .

Next, we quantified the degree of brittleness ( $m$ ) by measuring the slope of the  $G/G_0$  vs.  $\gamma$  curve beyond the yield strain  $\gamma_Y$  (shaded regions), as shown in Fig. S1(i)–(l) for the experiments. The same procedure has been adopted for the simulation data. To compare across different cases, the yielding slope was normalized by the maximum slope  $m_{\text{max}}$  in a given scenario, defining the normalized degree of brittleness as  $\tilde{m} = m/m_{\text{max}}$ .

## S2 Yielding under symmetric shear:

We examine the yielding behavior of the sample trained under a symmetric shear training protocol, where the applied strain follows the sequence  $(0 \rightarrow \gamma_T \rightarrow 0 \rightarrow -\gamma_T \rightarrow 0)$  (the protocol is shown in Fig. S2(a) for the positive-direction readout). The tunability of the yield point persists in this case as well. Fig. S2(b) shows the variation of  $|\gamma_Y|$  with  $|\gamma_T|$  for both positive and negative direction readouts. Fig. S2(c) and (d) display the typical behavior of  $G/G_0$  as a function of  $\gamma$  for the positive and negative direction readouts, respectively.

## S3 Un-normalized mean non-affinity during readout:

The mean non-affinity,  $\overline{\Delta(x,y)}$ , computed from the non-affinity map  $\Delta(x,y)$  for three representative  $\gamma_T$  values, is shown in Fig. S3(a). The system trained with a larger  $\gamma_T$  exhibits a higher initial non-affinity. However, in all cases, the non-affinity increases from its baseline value once the applied strain exceeds the corresponding  $\gamma_T$ . Fig. S3(b) shows the mean non-affinity for various  $\gamma_T$  values, while Fig. S3(c) presents the unnormalized mean non-affinity as a colormap for all training amplitudes during the readouts.

## S4 Non-affinity map during readout for various $\gamma_T$ :

In the main text, we presented the non-affinity maps during readout for the system trained at  $\gamma_T = 0.10$  at three representative strain values. Here, in Fig. S4, we show the non-affinity maps during readouts for systems trained with different  $\gamma_T$  values, covering a broader range of strain points to illustrate the evolution of the spatial non-affinity in greater detail.

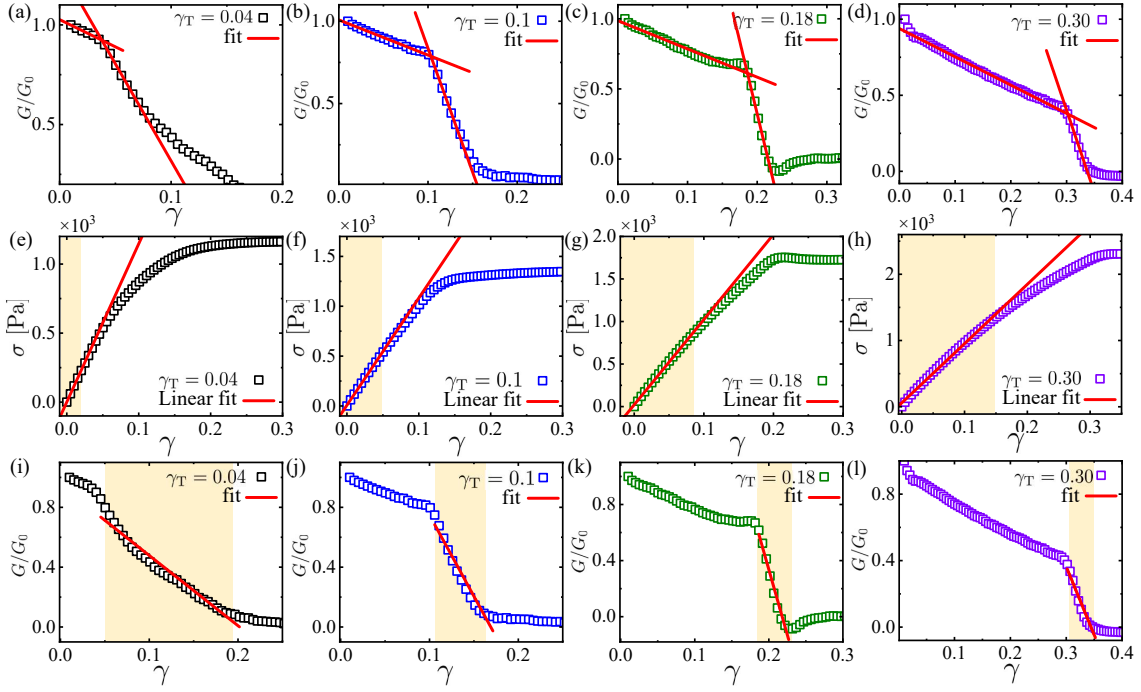

Figure S1: **Top panel:** (a) to (d) show the analysis by which we predict the training strain amplitude from the corresponding read out responses for  $\gamma_T = 0.04, 0.1, 0.18$  and  $0.30$ . **Middle panel:** (e) to (h) Show how we calculate the linear modulus in each case. The shaded regions corresponds the  $\gamma$  range (up to  $\gamma_Y/2$ ) we select to compute the slope. **Bottom panel:** (i) to (l) Show the overall yielding slope in each case. The shaded areas correspond to the chosen regions to calculate the slopes.

## S5 Mechanical properties of thermally annealed systems from our simulation:

Similar to the main text Fig. 3(d)–(f), where we used thermally annealed data from Ref.[9] from the main text, here we present the corresponding results obtained from our simulations. The mechanical properties of both thermally and mechanically annealed systems are shown for comparison. The thermally annealed data from our simulations exhibit a similar trend as observed previously, confirming the consistency of the mechanical response across different datasets.

## S6 Correlation between $E_{IS}$ and $\tilde{m}$ (simulation):

Fig. S6 shows that the brittleness  $\tilde{m}$  decreases with increasing  $E_{IS}$  in both the cases (TA and MA). To quantify this trend, we calculated the Pearson correlation coefficient (PCC) between  $E_{IS}$  and  $\tilde{m}$ . We find a strong negative correlation for both protocols:  $PCC \approx -0.8255$  (for MA) and  $PCC \approx -0.8987$  (for TA).

## S7 Calculating Young's modulus $E$ and defining the yield stress $\sigma_Y$ :

### S7.1 Experiments:

We first determine the Poisson ratio  $\nu$ . Axial (tensile) deformation is applied to the sample, and the corresponding lateral displacement is measured. From the ratio of lateral to axial strain, we obtain  $\nu \approx 0.41$ . Using this value, the Young's modulus for each training amplitude  $\gamma_T$  is calculated as  $E = 2G_{\text{linear}}(1 + \nu)$ , where  $G_{\text{linear}}$  is the linear shear modulus extracted as described in the section

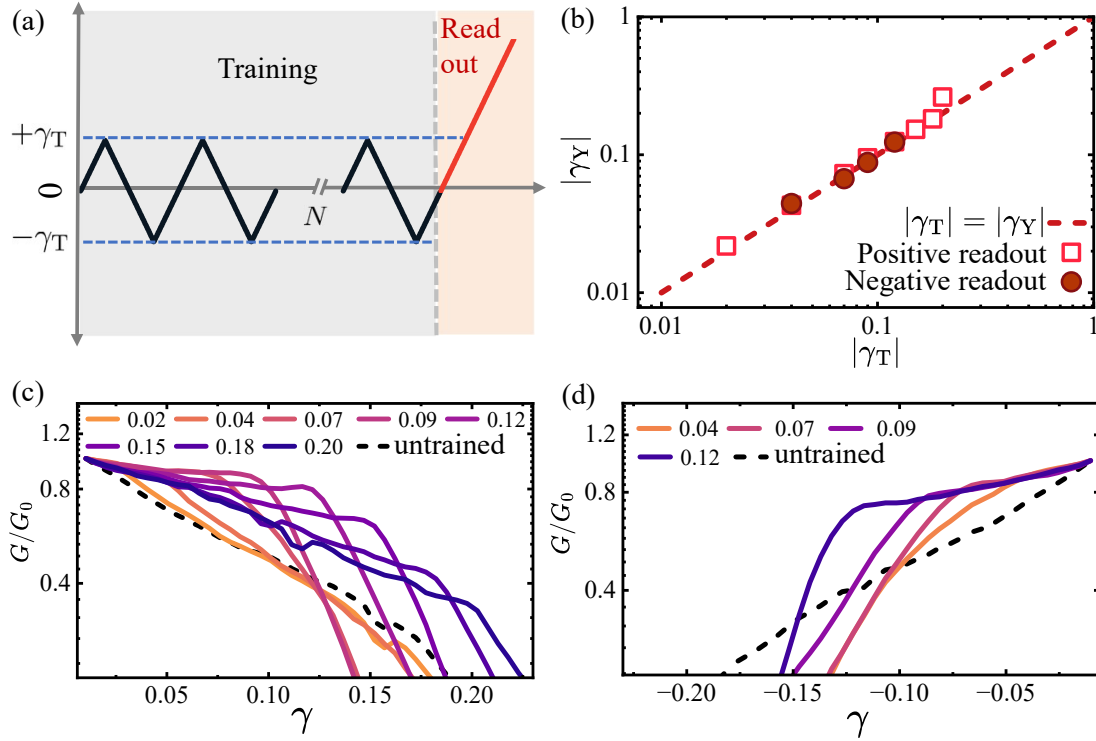

Figure S2: (a) Schematic of the protocol for symmetric shear strain perturbations where the readout is only in the positive direction. (b) The yield strain  $|\gamma_Y|$  versus training amplitude  $|\gamma_T|$  shows strong correlation as described in the main text. The normalised differential shear modulus as a function of deformation  $\gamma$  during the readout for the readout (c) in the positive direction and (d) in the negative direction respectively, where the samples are prepared via symmetric training cycles.

S1. The yield stress  $\sigma_Y$  is defined as the stress evaluated at the experimentally determined yield strain  $\gamma_Y$ .

## S7.2 Simulations:

In the case of MA, we first compute the bulk modulus  $K$  for each training amplitude  $\gamma_T$ . The Young's modulus is then obtained using the standard relation  $E = \frac{9KG_{\text{linear}}}{3K + G_{\text{linear}}}$ . The yield stress  $\sigma_Y$  in simulations is defined analogously to the experiments, i.e., the stress evaluated at the yield strain  $\gamma_Y$ .

To calculate Young's modulus in the case of TA, we used the Poisson ratio  $\nu \approx 0.42$  (which is obtained by using the shear modulus  $G_{\text{linear}}$ , and bulk modulus  $K$  mentioned above).

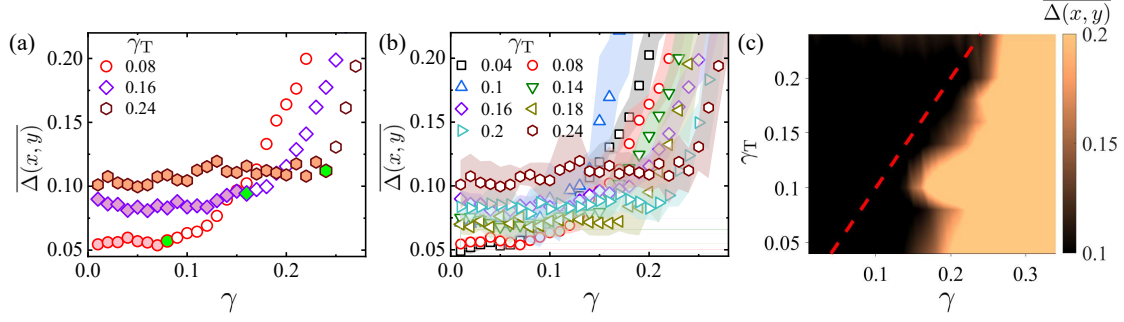

Figure S3: (a) The un-normalized mean non-affinity during readout for trained systems, with  $\gamma_T = 0.08, 0.16$  and  $0.24$ , in every case the training amplitudes are marked by the green symbols. (b) Shows the mean non-affinity during readout for all the trained systems. The shaded regions in all cases are the standard deviations of the data points. (c) The un-normalized mean non-affinity during readouts  $\overline{\Delta(x, y)}$  are plotted as the color map for various  $\gamma_T$ , same as main Fig. (2)(a).

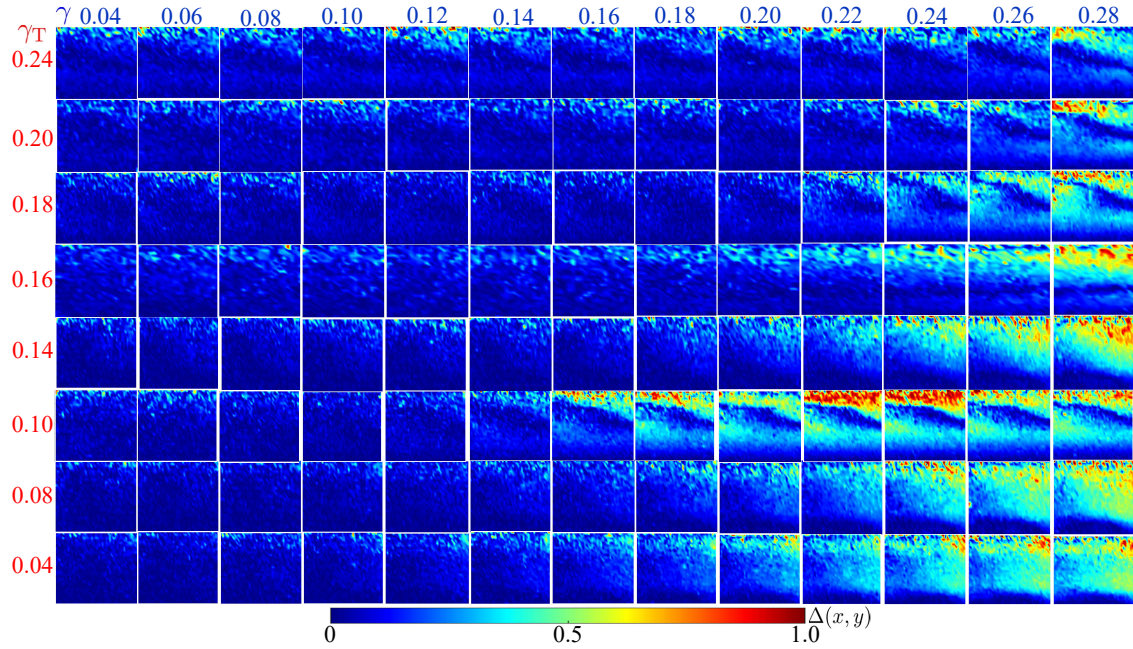

Figure S4: The non-affine maps during readout for all the systems at different readout deformation ( $\gamma$ ) and training amplitudes  $\gamma_T$ , placed along the horizontal and the vertical direction, respectively.

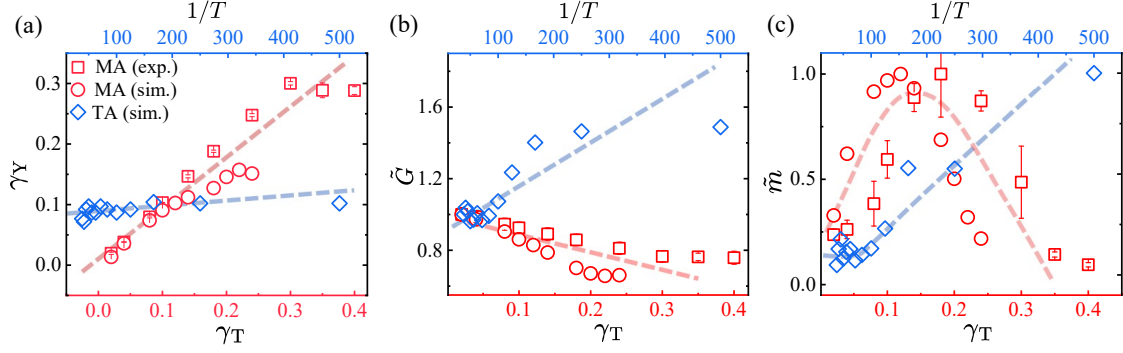

Figure S5: (a) Yield strain  $\gamma_Y$ , (b) normalized linear modulus  $\tilde{G}$ , and (c) normalized brittleness  $\tilde{m}$  are plotted for both thermally and mechanically annealed systems. Blue diamond symbols represent thermal annealing data from our simulation, red squares and circles correspond to mechanical annealing in experiments and simulation respectively. In all panels, red and blue dashed lines are guides to the eye for mechanical and thermal annealing trends, respectively.

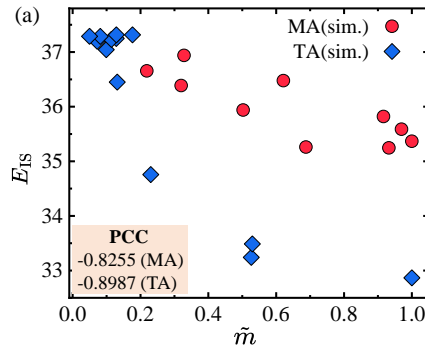

Figure S6: (a)  $E_{IS}$  is plotted with  $\tilde{m}$  for both mechanically and thermally annealed systems. The red circles and the blue diamonds represent the data for MA and TA respectively. Pearson Correlation Coefficient (PCC) are mentioned in the inset for both the cases.
